# Supplementary material for: WOT-Class: Weakly Supervised Open-world Text Classification
Source: arXiv:2305.12401 source file (2023-11-22)
Supplement: Supplementary file 1 [file 7-appendix.tex]

\iffalse
\section{Implementation Details}\label{app:1}

\subsection{Implementation Details of \our}
In our experiments, we fine-tune the pre-trained BERT-base-uncased model provided in Huggingface’s \texttt{Transformers} library~\cite{wolf2019huggingface}.
In our framework, we start with $K=100$ initial classes. For a cluster $i$, we fix $W=50$ to get sufficient statistically representative words to provide MLP features.
In class-word ranking, the quality ratio threshold is $\beta=0.7$.
The analysis of hyper-parameter sensitivity is shown in Sec.~\ref{sec:4.4}.

\subsection{Computational Budget}
All experiments are conducted using a 32-Core Processor and a single RTX A6000 GPU.
The expected running time of \our is less than one hour, for a dataset with a sample size of 10,000 (e.g., 20News).
%A larger dataset may require more time; for DBpedia (a massive dataset with 560,000 samples), 10 hours is expected. Note, however, that ORCA cannot provide same-condition results in a single day.

\begin{figure*}[t]
\begin{center}
\subfigure[20News]{
    \includegraphics[width =.3\linewidth]{graph.pdf}
}
\subfigure[NYT]{
    \includegraphics[width =.3\linewidth]{graph-NYT.pdf}
}
\subfigure[AGNews]{
    \includegraphics[width =.3\linewidth]{graph-AG.pdf}
}
\caption{Sensitivity on the Initial Guessed Number of Classes for 20News, NYT and AGNews. The mean macro-F$_1$ scores over three runs are reported. \our is slow on DBpedia, therefore not reported.}
\label{Fig.app}
\end{center}
\end{figure*}
\fi

\section{Additional Results}\label{app:results}
%We additionally show the micro-F$_1$ scores of experiments, the prediction of the class number, and the full list of the class nomination in Sec.~\ref{sec:exp}.
%We additionally show more experimental results.

\iffalse
\smallsection{Effect of Extra Classifier}
To verify the effectiveness of the extra classifier (see details in Appendix~\ref{app:1}) after the iterative refinement, we design \our-GMM which obtains the labels from the GMM in the last iteration.
The improvement of \our over \our-GMM in Table~\ref{table:GMM} shows the usefulness of the classifier training.

\smallsection{Imbalance Tolerance}
We further show the performance of ORCA and \our on imbalanced DBpedia for both seen and unseen classes.

As shown in Figure~\ref{Fig.app2}, ORCA's performance drops more than 40\% on unseen classes, demonstrating its intolerance to imbalanced data distributions.

\begin{figure*}[t]
\begin{center}
\subfigure[seen]{
    \includegraphics[width =.3\linewidth]{imbalance-seen.pdf}
}
\subfigure[unseen]{
    \includegraphics[width =.3\linewidth]{imbalance-unseen.pdf}
}
\caption{Performance of ORCA and \our on different imbalance degrees.}
\label{Fig.app2}
\end{center}
\end{figure*}
\fi

\smallsection{Performance of the Seen and Unseen Classes}
Table~\ref{table:app} and \ref{table:app_} show the micro/macro-F$_1$ scores of seen and unseen classes as a supplement to Table~\ref{table:1}.

\smallsection{Imbalance Tolerance}
Table~\ref{tab:per-im} shows the macro-F$_1$ scores of the overall, seen, and unseen performance of \our and compared methods.

\iffalse
\smallsection{Examples of Class-words}
We additionally show the full list of the final class-words we selected for unseen clusters on two datasets. As shown in Table~\ref{table:app4}, our class-words are highly related to (or even as same as) ground truth class names and human-understandable.

\smallsection{Robustness of the framework}
In the paper, we have shown \our framework with CGExpan and X-Class worked well on 7 datasets with different hyperparameters. We further clarify that we use them as routines,  so they can be replaced by other similar functioning methods. For example, we replace CGExpan with a novel method \textbf{GAPA}~\cite{li2022automatic}, and show the result on 2 datasets in Table~\ref{table:gapa}. This indicates the flexibility of our method to suit new works.
\fi

\iffalse
\begin{table*}[h!]
  \begin{center}
    \caption{Performance of \our with different entity set expansion methods.}\label{table:gapa}{
    \begin{tabular}{c  c  c  c}
      \toprule
      \textbf{Method} & \textbf{AGNews} & \textbf{NYT-S} &  \textbf{DBpedia} \\
       \midrule
       \our (CGExpan) & 13.16/10.62 & 26.21/20.56 & 2.68/1.96\\
       \our (GAPA) & / & / & / \\
      \bottomrule
    \end{tabular}}
  \end{center}
\end{table*}
\fi
